# Supplementary material for: Dynamical analysis of quantum matter bounces with dark sector mimickers
Source: arXiv:2501.04749 source file (2025-01-08)
Supplement: Supplementary file 1 [file appendix1.tex]

\section{Appendix} \label{sec:appendix}
